# Supplementary material for: Strong Exciton-Photon Coupling in a Nanographene Filled Microcavity
Source: arXiv:1709.04499 source file (2017-09-13)
Supplement: Supplementary file 1 [file SI-Strong_Exciton-Photo_Coupling_in_a_Nanographene_Filled_Microcavity.pdf]

# Supplementary Information

# for

## Strong Exciton-Photon Coupling in a Nanographene Filled Microcavity

By

D M Coles[1], Q Chen[2], L C Flatten[3], J M Smith[3], K Müllen[2], A Narita[2] and D G Lidzey[1]

1) Department of Physics & Astronomy, University of Sheffield, Sheffield S3 7RH, UK

2) Max Planck Institute for Polymer Research, Mainz D-55128, Germany

3) Department of Materials, University of Oxford, Oxford OX1 3PH, UK

Correspondence and requests for materials should be addressed to D G Lidzey (email: d.g.lidzey@sheffield.ac.uk) or to K Müllen (email: muellen@mpip-mainz.mpg.de) or to A Narita (email: narita@mpip-mainz.mpg.de).

# Table of Content

Methods .......... 3

General methods .......... 3

Synthetic details .......... 3

NMR and MS Spectra .......... 12

References .......... 21

# Methods

## General methods

All reactions working with air- or moisture- sensitive compounds were carried out under argon atmosphere using standard Schlenk line techniques. Unless otherwise noted, all starting materials, solvents, and reagents were purchased from commercial sources and used without further purification. Thin layer chromatography (TLC) was done on silica gel coated aluminum sheets with F254 indicator and column chromatography separation was performed with silica gel (particle size 0.063-0.200 mm). Melting points were determined on a Büchi hot stage apparatus and were uncorrected. Nuclear Magnetic Resonance (NMR) spectra were recorded using Bruker DPX 250, Bruker DPX 300, and Bruker DPX 700 MHz NMR spectrometers. Chemical shifts ($\delta$) were expressed in ppm relative to the residual of solvent. Coupling constants ($J$) were recorded in Hertz. Field desorption mass (FD-MS) spectra were measured using a VG instruments ZAB 2-SE-FPD using 8 kV accelerating voltage. High resolution mass spectra (HRMS) were recorded on a Bruker Reflex II-TOF spectrometer by matrix-assisted laser decomposition/ionization (MALDI) using 7,7,8,8-tetracyanoquinodimethane (TCNQ) as matrix.

## Synthetic details

**DBOV-Mes** was synthesized as shown in Scheme S1, adapting and partially improving a procedure we have recently reported[1,2]. Starting materials **1**[1] and **2**[2] were prepared according to reported procedures.

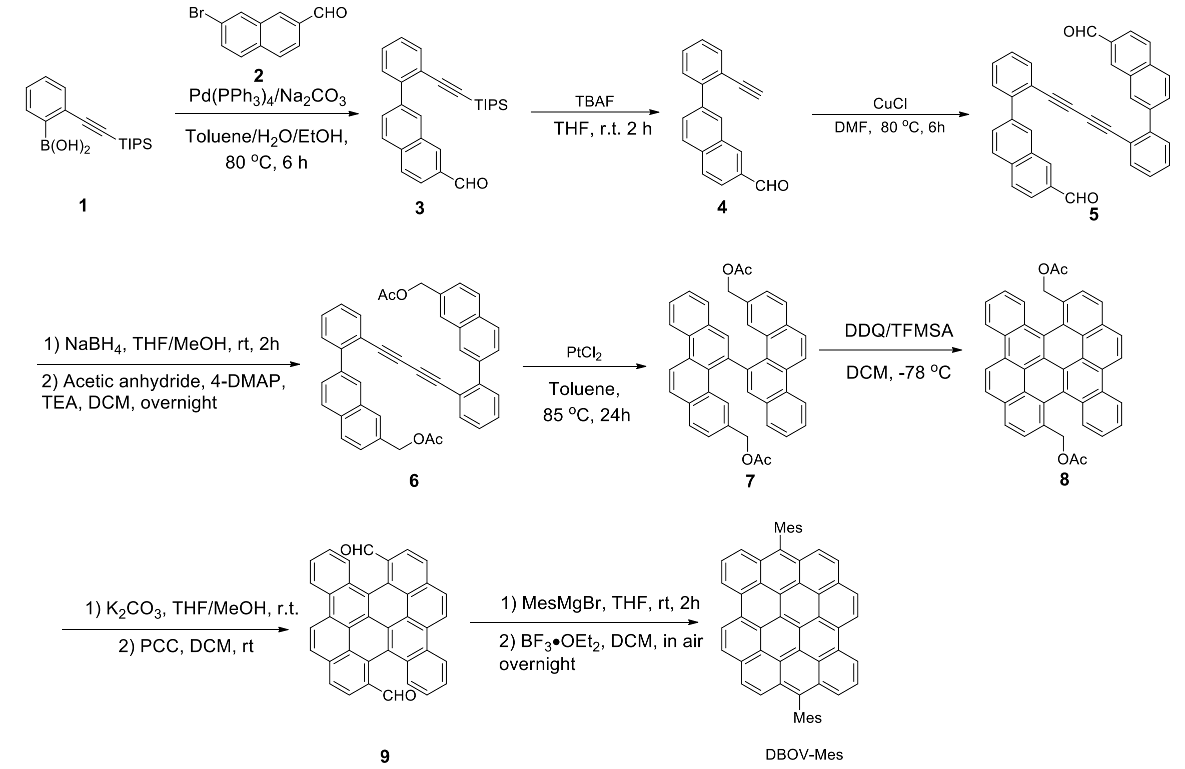


**Scheme S1.** Synthetic route towards **DBOV-Mes**.

## **7-(2-((Triisopropylsilyl)ethynyl)phenyl)-2-naphthaldehyde (3)**:

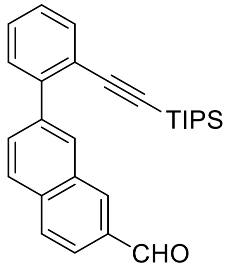


To a 250-mL Schlenk flask were added (2-((triisopropylsilyl)ethynyl)phenyl)boronic acid **1** (2.12 g, 7.02 mmol), 7-bromo-2-naphthaldehyde **2** (1.20 g, 6.38 mmol), and $Na_2CO_3$ (2.23 g, 21.1 mmol). The flask was evacuated and backfilled with Ar for 3 times. Then toluene/EtOH/$H_2O$ = 4:1:1 (72 mL/18 mL/18 mL) was added via a syringe. After degassed by bubbling with Ar for 15 min, $Pd(PPh_3)_4$ (369 mg, 0.319 mmol) was added in one portion. The mixture was then heated at 80 °C for 6 h under Ar atmosphere. After completion of the reaction, the mixture was cooled down to room temperature and

extracted with ethyl acetate (50 mL) for 3 times. The combined organic layers were washed with brine (80 mL), dried over $Na_2SO_4$, and evaporated. The residue was purified by silica gel column chromatography (*n*-hexane/ethyl acetate = 10 : 1) to give the title compound (2.80 g, 97% yield) as colorless oil. TLC $R_f$ = 0.5 (*n*-hexane/ethyl acetate = 10 : 1); $^1$H NMR (250 MHz, $CD_2Cl_2$) $\delta$ 10.16 (s, 1H), 8.30 (d, $J$ = 33.5 Hz, 2H), 8.04 – 7.82 (m, 4H), 7.73 – 7.59 (m, 2H), 7.54 – 7.20 (m, 3H), 1.03 – 0.90 (m, 21H); $^{13}$C NMR (75 MHz, $CDCl_3$) $\delta$ 192.4, 143.5, 139.7, 135.8, 135.1, 134.4, 134.0, 132.6, 131.2, 129.9, 129.6, 128.9, 128.8, 127.7, 127.6, 122.9, 122.4, 106.2, 94.8, 18.6, 11.3. FD-MS (8 kV): *m*/*z* 412.9; HRMS (MALDI-TOF): *m*/*z* Calcd for $C_{28}H_{30}OSi$: 413.2295 $[M+H]^+$, found: 413.2302.

## 7-(2-Ethynylphenyl)-2-naphthaldehyde (4):

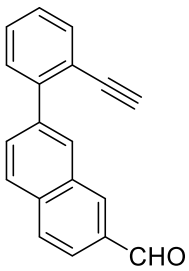


To a solution of 7-(2-((triisopropylsilyl)ethynyl)phenyl)-2-naphthaldehyde (**3**) (2.80 g, 6.78 mmol) in anhydrous tetrahydrofuran (THF) (50 mL) was added tetra-*n*-butylammonium fluoride (TBAF) (6.78 mmol, 6.78 mL, 1.00 M in THF) dropwise, and the mixture was stirred at room temperature for 2 h. After completion of the reaction, MeOH (10 mL) was added followed by stirring for another 30 min. Then the mixture was diluted with ethyl acetate (100 mL), washed with water (50 mL) and brine (50 mL), dried over $Na_2SO_4$, and evaporated. The residue was purified by silica gel column chromatography (*n*-hexane/ethyl acetate = 10 : 1) to yield the title compound (1.6 g, 92%) as white solid. TLC $R_f$ = 0.2 (*n*-hexane/ethyl acetate = 10 : 1); Mp: 93.7 – 94.1 °C; $^1$H NMR (300 MHz, $CD_2Cl_2$) $\delta$ 10.17 (s, 1H), 8.41 (s, 1H), 8.22 (s, 1H), 8.05 – 7.96 (m, 3H), 7.95 – 7.86 (m, 1H), 7.73 – 7.65 (m, 1H), 7.57 – 7.46 (m, 2H), 7.45 – 7.33 (m, 1H), 3.12 (s, 1H); $^{13}$C NMR (75 MHz, $CD_2Cl_2$) $\delta$ 192.4, 135.0, 135.0, 134.4, 131.1, 130.2, 130.1,

129.7, 129.2, 128.0, 128.0, 123.4, 83.2, 80.9; FD-MS (8 kV): *m*/*z* 256.6; HRMS (MALDI-TOF): *m*/*z* Calcd for $C_{19}H_{12}O$: 256.0888 $[M]^+$, found: 256.0868.

## 1,4-Bis(2-(7-formylnaphthalen-2-yl)phenyl)buta-1,3-diyne (5):

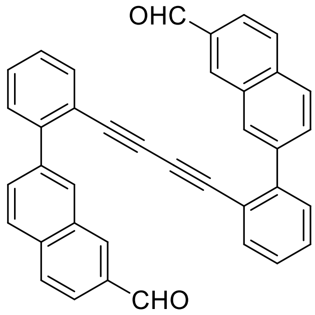


To a solution of 7-(2-ethynylphenyl)-2-naphthaldehyde (**4**) (1.60 g, 6.24 mmol) in dry *N*,*N*-dimethylformamide (16 mL) was added CuCl (620 mg, 6.24 mmol). The mixture was heated at 80 °C under air for 12 h. After completion of the reaction, the mixture was cooled down to room temperature, and then diluted with ethyl acetate (100 mL) and washed with 1 N HCl (50 mL). The aqueous phase was extracted with ethyl acetate (30 mL) for 3 times. The combined organic layers were washed with saturated solution of $Na_2CO_3$ (60 mL), brine (60 mL), dried over $Na_2SO_4$, and concentrated in vacuo. The precipitated solid was collected by filtration and washed with cold methanol (30 mL) to give compound **5** (1.34 g, 98%) as a white solid. TLC $R_f$ = 0.2 (*n*-hexane/ethyl acetate = 4 : 1); Mp: 206.1 – 206.9 °C; $^1$H NMR (300 MHz, $CD_2Cl_2$) $\delta$ 10.10 (s, 1H), 8.32 (s, 1H), 8.13 (s, 1H), 7.98 – 7.90 (m, 2H), 7.88 – 7.81 (m, 2H), 7.68 – 7.57 (m, 1H), 7.53 – 7.45 (m, 1H), 7.42 – 7.30 (m, 1H); $^{13}$C NMR (75 MHz, $CD_2Cl_2$) $\delta$ 192.3, 144.5, 139.2, 136.0, 135.0, 134.9, 134.7, 132.9, 130.8, 130.3, 130.1, 129.9, 129.2, 128.1, 128.0, 123.4, 120.5, 81.9, 77.1; FD-MS (8 kV): *m*/*z* 510.6; HRMS (MALDI-TOF): *m*/*z* Calcd for $C_{38}H_{22}O_2$: 510.1620 $[M]^+$, found: 510.1587.

**1,4-Bis(2-(7-diacetoxymethylnaphthalen-2-yl)phenyl)buta-1,3-diyne (6)**:

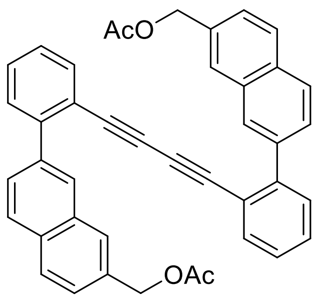


To a solution of 1,4-bis(2-(7-formylnaphthalen-2-yl)phenyl)buta-1,3-diyne (**5**) (900 mg, 1.76 mmol) in a mixture of THF (150 mL) and methanol (30 mL) was added $NaBH_4$ (200 mg, 5.29 mmol). The mixture was stirred at room temperature for 1 h. After completion of the reaction, acetone (10 mL) was added into the mixture and stirred for 10 min. The solvents were evaporated and the residue was redissolved in ethyl acetate (50 mL), and washed with water (50 mL), brine (50 mL), and dried over $Na_2SO_4$. The solvent was tehn removed in vacuo to obtain a diol intermediate (892 mg, 99% yield) as a white solid. The diol intermediate (892 mg, 1.73 mmol) was redissolved in anhydrous dichloromethane (150 mL), and then triethylamine (534 mg, 5.28 mmol), 4-dimethylaminopyridine (65 mg, 0.53 mmol), and acetic anhydride (539 mg, 5.28 mmol) were added. The mixture was stirred at room temperature for 2 h. After completion of the reaction, the solvent was evaporated and the residue was purified by column chromatography over silica gel (*n*-hexane/ethyl acetate = 10 : 1) to give compound **6** (912 mg, 87% yield) as a white solid. TLC $R_f$ = 0.3 (*n*-hexane/ethyl acetate = 10 : 1); Mp: 60.0 – 60.5 °C; $^1$H NMR (300 MHz, $CD_2Cl_2$) $\delta$ 8.02 (d, *J* = 1.7 Hz, 2H), 7.94 – 7.86 (m, 4H), 7.82 (d, *J* = 8.5 Hz, 2H), 7.74 (dd, *J* = 8.5, 1.8 Hz, 2H), 7.69 – 7.61 (m, 2H), 7.58 – 7.45 (m, 6H), 7.38 (ddd, J = 7.7, 6.6, 2.2 Hz, 2H), 5.29 (s, 4H), 2.13 (s, 6H). $^{13}$C NMR (75 MHz, $CD_2Cl_2$) $\delta$ 171.0, 145.1, 138.4, 134.6, 134.6, 133.4, 132.7, 130.2, 130.0, 128.4, 128.0, 127.8, 127.7, 127.6, 126.6, 120.5, 81.9, 76.9, 66.6, 21.2; FD-MS (8 kV): *m*/*z* 597.0; HRMS (MALDI-TOF): *m*/*z* Calcd for $C_{42}H_{30}O_4$: 598.2144 $[M]^+$, found: 598.2115.

**3,3'-Diacetoxymethyl-5,5'-bichrysene (7)**:

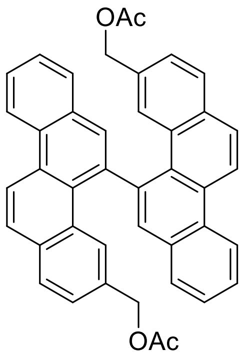


1,4-Bis(2-(7-diacetoxymethylnaphthalen-2-yl)phenyl)buta-1,3-diyne (**6**) (800 mg, 1.34 mmol) and $PtCl_2$ (89.0 mg, 0.334 mmol) in a 250-mL Schlenk flask was dried under vacuum for 1 h, and then the apparatus was evacuated and backfilled with Ar for 3 times before anhydrous toluene (80 mL) was added. The mixture was degassed by three freeze-pump-thaw cycles and then heated at 90 °C for 60 h. The reaction was monitored by $^1$H NMR. After completion of the reaction, the mixture was cooled down to room temperature and the solvent was evaporated. The resulting yellow brown residue was purified by column chromatography over silica gel (*n*-hexane/ethyl acetate = 10 : 1) to give the title compound (260 mg, 33% yield) as a white solid. TLC $R_f$ = 0.3 (*n*-hexane/ethyl acetate = 4 : 1); Mp: 196.2 – 196.9 °C; $^1$H NMR (300 MHz, $CD_2Cl_2$) $\delta$ 9.00 – 8.87 (m, 4H), 8.14 – 8.04 (m, 4H), 7.93 – 7.82 (m, 6H), 7.81 – 7.72 (m, 2H), 7.70 – 7.60 (m, 2H), 7.30 – 7.22 (m,, 2H), 4.51 – 4.34 (m, 4H), 1.23 (s, 6H). $^{13}$C NMR (75 MHz, $CD_2Cl_2$) $\delta$ 170.4, 130.7, 128.7, 128.4, 127.4, 127.4, 126.8, 125.6, 123.7, 122.3, 66.0, 20.0; FD-MS (8 kV): *m*/*z* 598.3; HRMS (MALDI-TOF): *m*/*z* Calcd for $C_{42}H_{30}O_4$: 598.2144 $[M]^+$, found: 598.2345.

**5,14-Diacetoxymethylbenzo[*a*]dinaphtho[2,1,8-*cde*:1',2',3',4'-ghi]perylene (8)**:

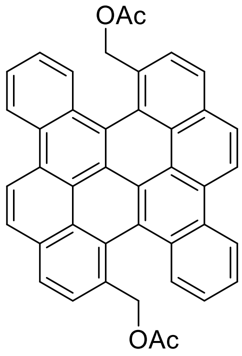


A solution of 3,3'-diacetoxymethyl-5,5'-bichrysene (**7**) (60 mg, 0.10 mmol) in dichloromethane (60 mL) was cooled down to –78 °C, and then trifluoromethanesulfonic acid (TFMSA) (0.6 mL) was added slowly via a syringe. The mixture was stirred for about 10 min to make the solution homogeneous, and then a solution of 2,3-dichloro-5,6-dicyano-1,4-benzoquinone (DDQ) (50 mg, 0.22 mmol) in anhydrous dichloromethane (6 mL) was added dropwise. The mixture was stirred at this temperature for another 2 h. After completion of the reaction, the mixture was poured into cold saturated aqueous solution of $Na_2CO_3$ (10 mL), and then extracted with dichloromethane (30 m) for 2 times. The combined organic layers were washed with brine (50 mL), dried over $Na_2SO_4$, and evaporated. The residue was purified by column chromatography over silica gel (*n*-hexane/ethyl acetate = 4 : 1) to give title compound (15 mg, 25% yield) as a yellow solid. TLC $R_f$ = 0.3 (*n*-hexane/ethyl acetate = 3 : 1); Mp: 281.1 – 282.7 °C; $^1$H NMR (250 MHz, $CD_2Cl_2$) $\delta$ 9.12 – 9.01 (m, 4H), 8.46 – 8.31 (m, 4H), 8.30 – 8.21 (m, 2H), 8.17 – 8.08 (m, 2H), 7.87 – 7.65 (m, 4H), 5.57 – 5.46 (m, 2H), 4.90 – 4.80 (m, J = 12.8, 1.8 Hz, 2H), 1.84 – 1.70 (m, 6H); $^{13}$C NMR (63 MHz, $CD_2Cl_2$) $\delta$ 170.7, 133.0, 131.2, 130.0, 129.0, 128.0, 127.9, 127.8, 127.6, 127.5, 127.1, 126.9, 126.5, 126.1, 125.5, 123.9, 122.3, 121.9, 66.4, 20.9; FD-MS (8 kV): *m*/*z* 594.9; HRMS (MALDI-TOF): *m*/*z* Calcd for $C_{42}H_{26}O_4$: 594.1831 $[M]^+$, found: 594.1823.

**5,14-Diformylbenzo[*a*]dinaphtho[2,1, 8-*cde*:1',2',3',4'-*ghi*]perylene (9)**:

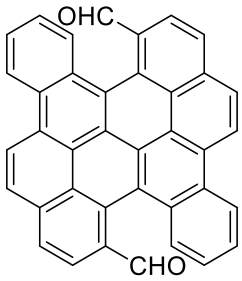


To a solution of 5,14-diacetoxymethylbenzo[*a*]dinaphtho[2,1,8-*cde*:1',2',3',4'-*ghi*]perylene (**8**) (60 mg, 0.10 mmol) in a mixture of dichloromethane (30 mL) and methanol (10 mL) was added $K_2CO_3$ (1.2 g, 8.7 mmol). The suspension was stirred at room temperature for 24 h. After completion of the reaction, the insoluble solid was filtered off and the filtrate was washed with water (20 mL), brine (20 mL), dried over $Na_2SO_4$, and evaporated. The residue was dried under vacuum using oil pump for 2 h. The obtained residue was redissolved in dry dichloromethane (40 mL), and then pyridinium chlorochromate (PCC) (80 mg, 0.37 mmol) was added in portions under vigorous stirring. The mixture was stirred for 2 h at room temperature, and methanol (1 mL) was added after confirming the completion of the reaction. The insoluble solid was filtered off and the filtrate was concentrated in vacuo. The residue was purified by column chromatography over silica gel (*n*-hexane/ethyl acetate = 4 : 1) to give title compound (30 mg, 59% yield in two steps) as red solid. TLC $R_f$ = 0.3 (*n*-hexane/EA = 4 : 1); Mp: >400 °C; $^1$H NMR (300 MHz, $C_2D_2Cl_4$) $\delta$ 9.46 (s, 2H), 9.01 (d, $J$ = 9.1 Hz, 2H), 8.90 (d, $J$ = 8.4 Hz, 2H), 8.52 – 8.42 (m, 4H), 8.34 (t, $J$ = 9.1 Hz, 4H), 7.83 – 7.72 (m, 2H), 7.64 (dd, $J$ = 8.1, 1.1 Hz, 2H); $^{13}$C NMR (75 MHz, $C_2D_2Cl_4$) $\delta$ 190.8, 133.7, 131.7, 131.6, 130.6, 128.5, 128.2, 127.9, 127.5, 127.1, 127.1, 125.9, 124.9, 124.4, 124.0, 123.9, 123.2, 121.2, 120.6; FD-MS (8 kV): *m*/*z* 506.9; HRMS (MALDI-TOF): *m*/*z* Calcd for $C_{38}H_{18}O_2$: 506.1307 $[M]^+$, found: 506.1293.

## 6,14-Dimesityldibenzo[*hi*,*st*]ovalene (DBOV-Mes):

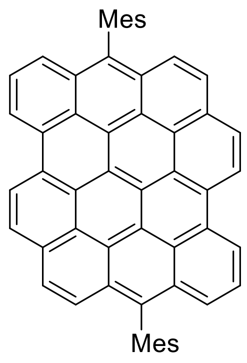


To a solution of 5,14-diformylbenzo[*a*]dinaphtho[2,1,8-*cde*:1',2',3',4'-*ghi*]perylene (**9**) (5 mg, 10 µmol) in anhydrous THF (5 mL) was added mesitylmagnesium bromide (0.15 mL, 150 µmol, 1.0 M in ether) dropwise under the protection of Ar. The mixture was stirred at room temperature for 2 h. After completion of the reaction, the yellow green colored solution was poured into saturated aqueous solution of $NH_4Cl$ (10 mL) and then extracted with ethyl acetate (20 mL) for 3 times. The combined organic layers were washed with brine (30 mL), dried over $Na_2SO_4$, and evaporated. After drying under vacuum using an oil pump for 2 h, the residue was redissolved in anhydrous dichloromethane (50 mL) and $BF_3 \cdot OEt_2$ (0.5 mL) was added using a syringe. The mixture was stirred at room temperature for 2 h. After completion of the reaction, the mixture was poured into saturated $NaHCO_3$ solution (10 mL). The organic phase was separated and dried over $Na_2SO_4$. The solvents were evaporated under reduced pressure and the residue was purified by column chromatography over silica gel (eluent: *n*-hexane/DCM = 10 : 1) to give **DBOV-Mes** (4 mg, 56%) as blue powder. TLC $R_f$ = 0.6 (*n*-hexane/ethyl acetate = 10 : 1); Mp: >400 °C; $^1$H NMR (700 MHz, *o*-dichlorobenzene-$d_6$) $\delta$ 9.33 (d, *J* = 7.8 Hz, 2H), 9.04 (d, *J* = 7.2 Hz, 2H), 8.44 (d, *J* = 7.4 Hz, 2H), 8.00 (d, *J* = 9.1 Hz, 2H), 7.98 (d, *J* = 8.3 Hz, 2H), 7.89 (t, *J* = 7.5 Hz, 2H), 7.78 (d, *J* = 9.0 Hz, 2H), 7.19 (s, 4H), 2.50 (s, 6H), 1.99 (s, 12H); FD-MS (8 kV): *m*/*z* 709.5; HRMS (MALDI-TOF): *m*/*z* Calcd for $C_{56}H_{36}$: 708.2817 $[M]^+$, found: 708.2814.

# NMR and MS Spectra

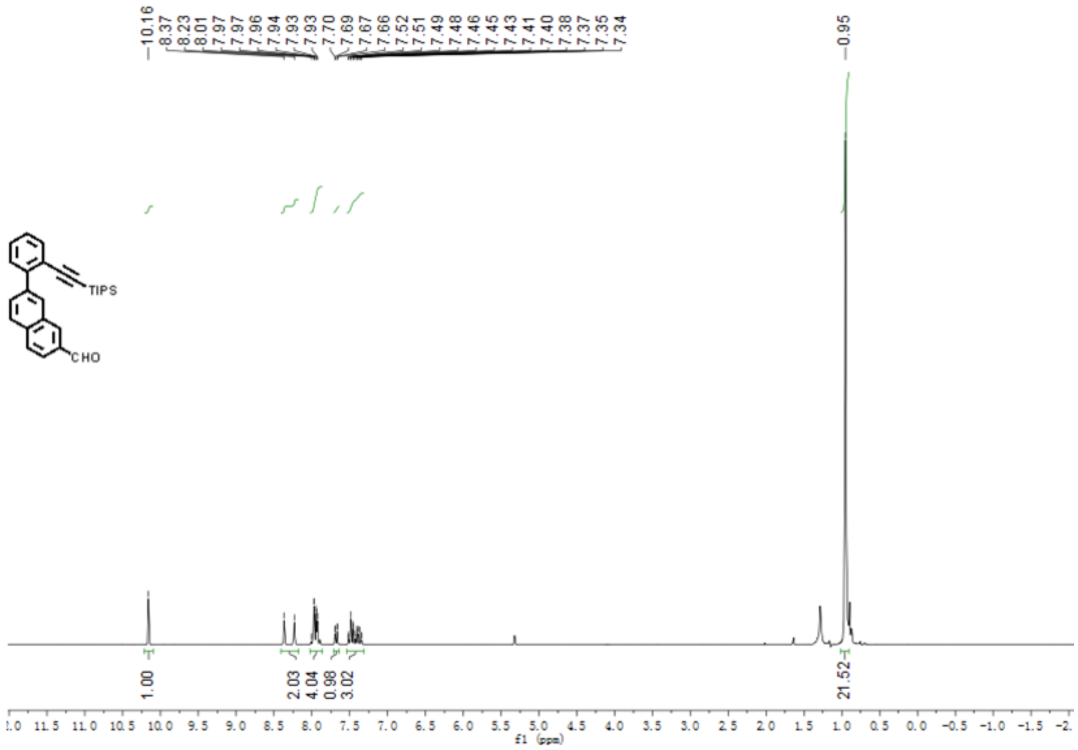

**Figure S1.** $^{1}H$ NMR spectra of compound **3** in $CD_2Cl_2$ (250 MHz, 298 K).

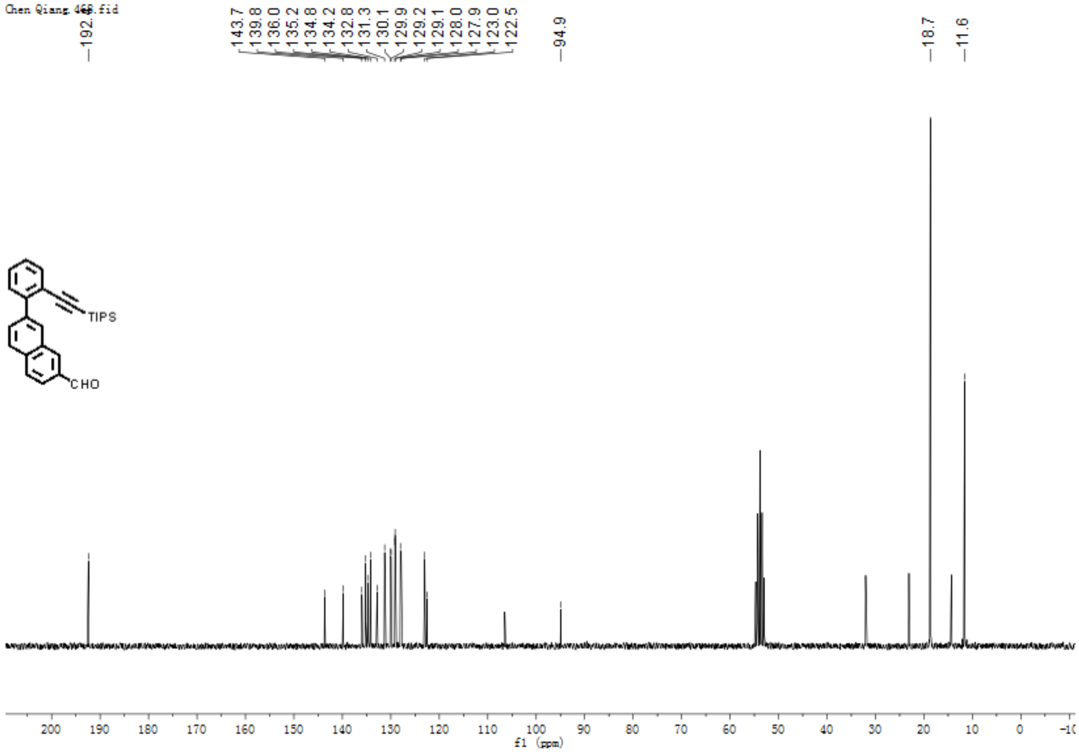

**Figure S2.** $^{13}C$ NMR spectra of compound **3** in $CD_2Cl_2$ (75 MHz, 298 K).

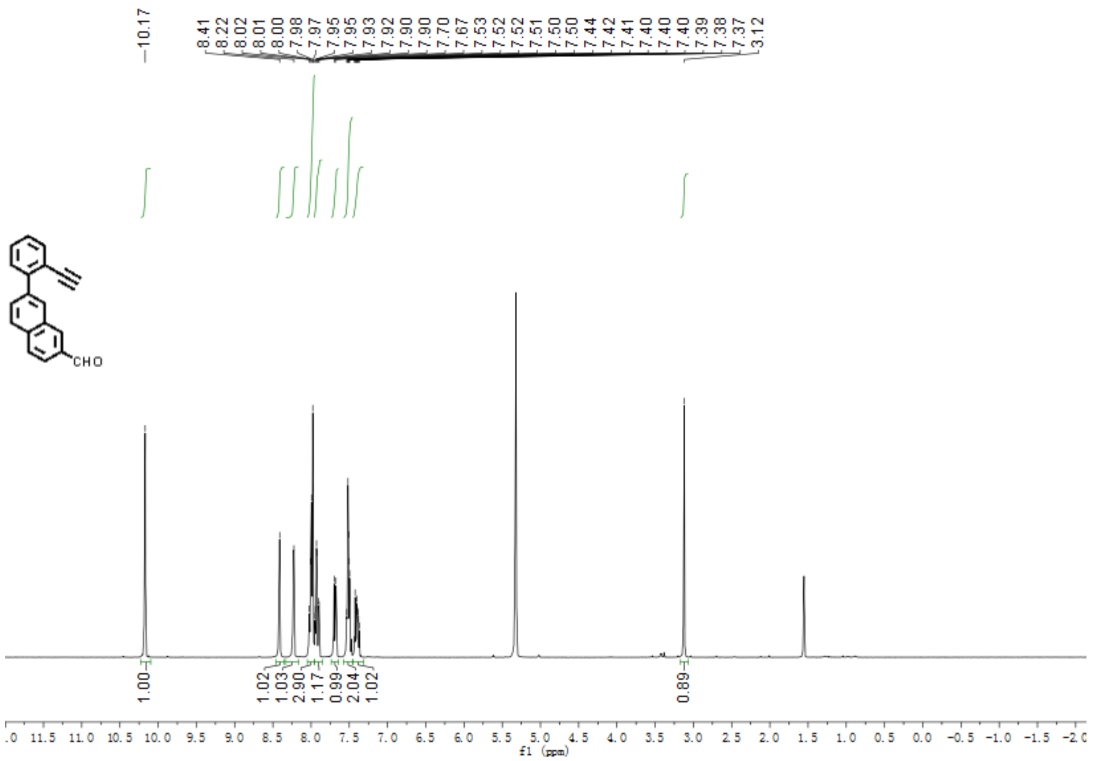


**Figure S3.** $^{1}$H NMR spectra of compound **4** in $CD_2Cl_2$ (300 MHz, 298 K).

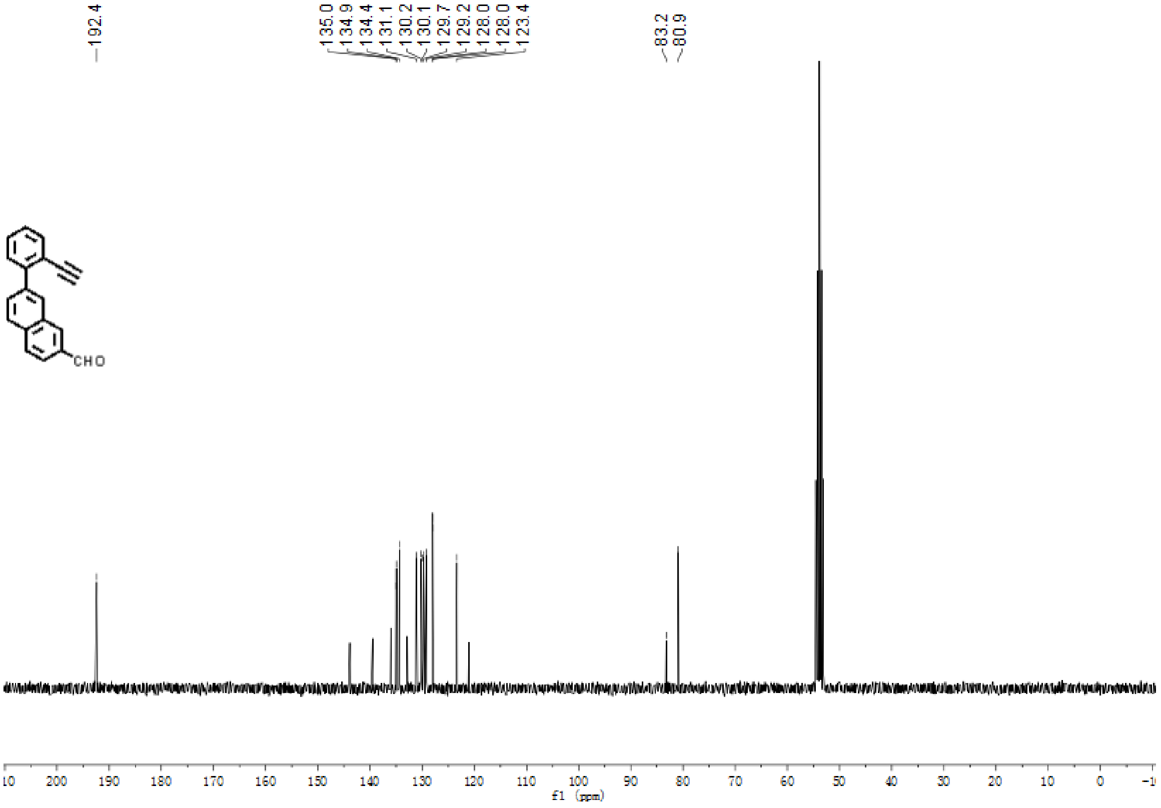


**Figure S4.** $^{13}$ C NMR spectra of compound **3** in $CD_2Cl_2$ (75 MHz, 298 K).

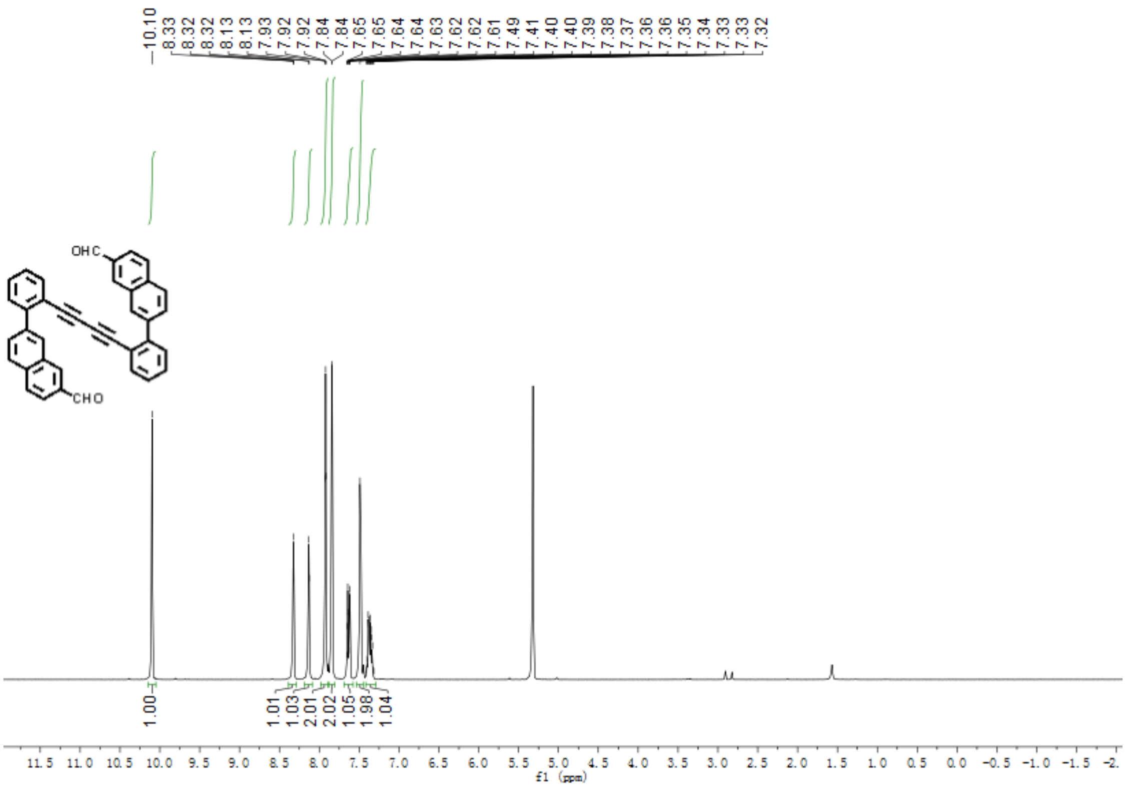


**Figure S5.** $^{1}$H NMR spectra of compound **5** in $CD_2Cl_2$ (300 MHz, 298 K).

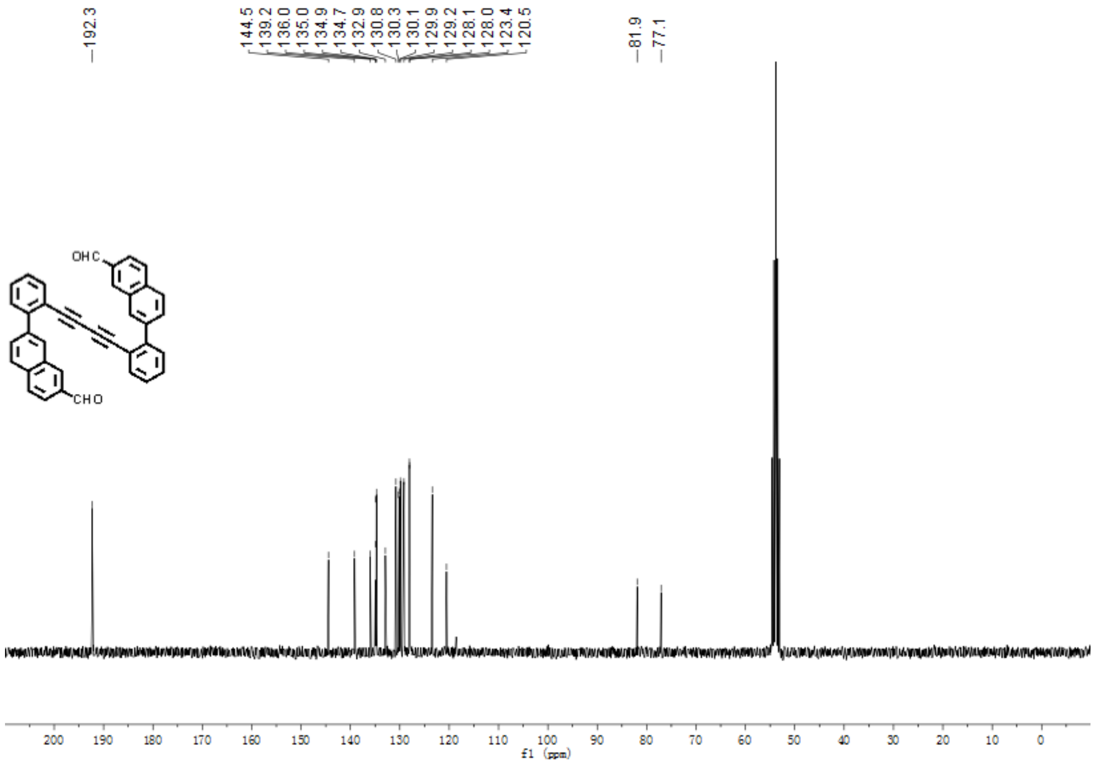


**Figure S6.** $^{13}$ C NMR spectra of compound **5** in $CD_2Cl_2$ (75 MHz, 298 K).

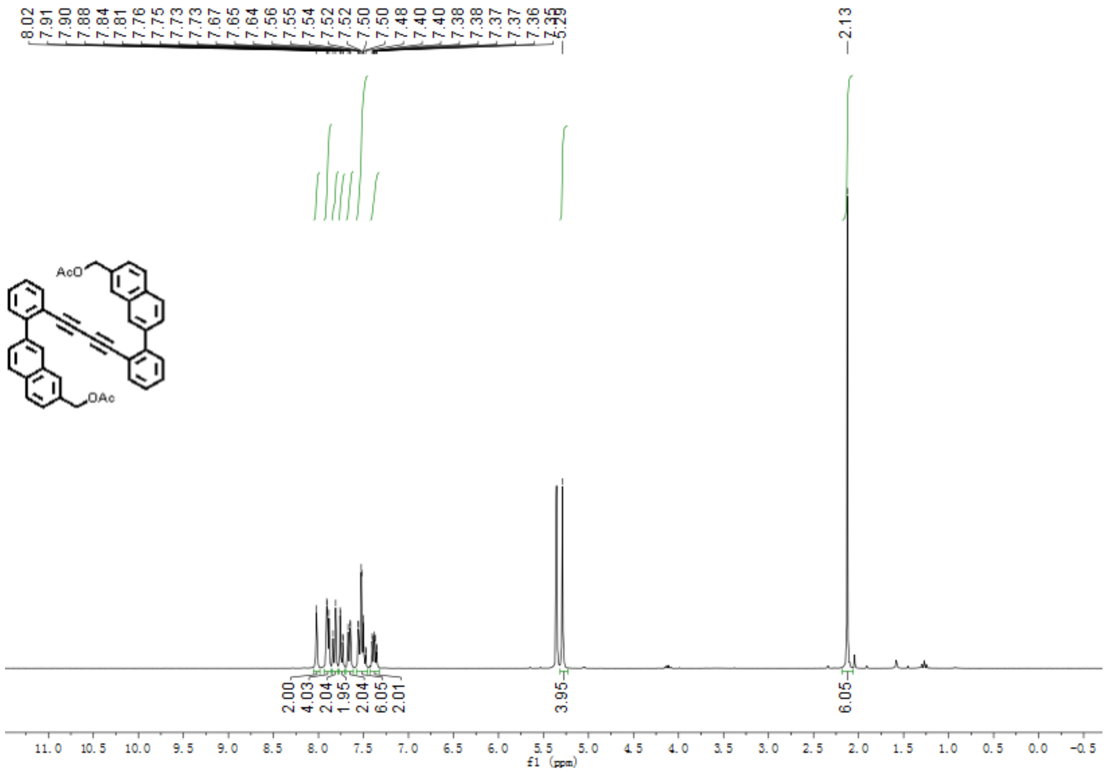


**Figure S7.** $^{1}$H NMR spectra of compound **6** in $CD_2Cl_2$ (300 MHz, 298 K).

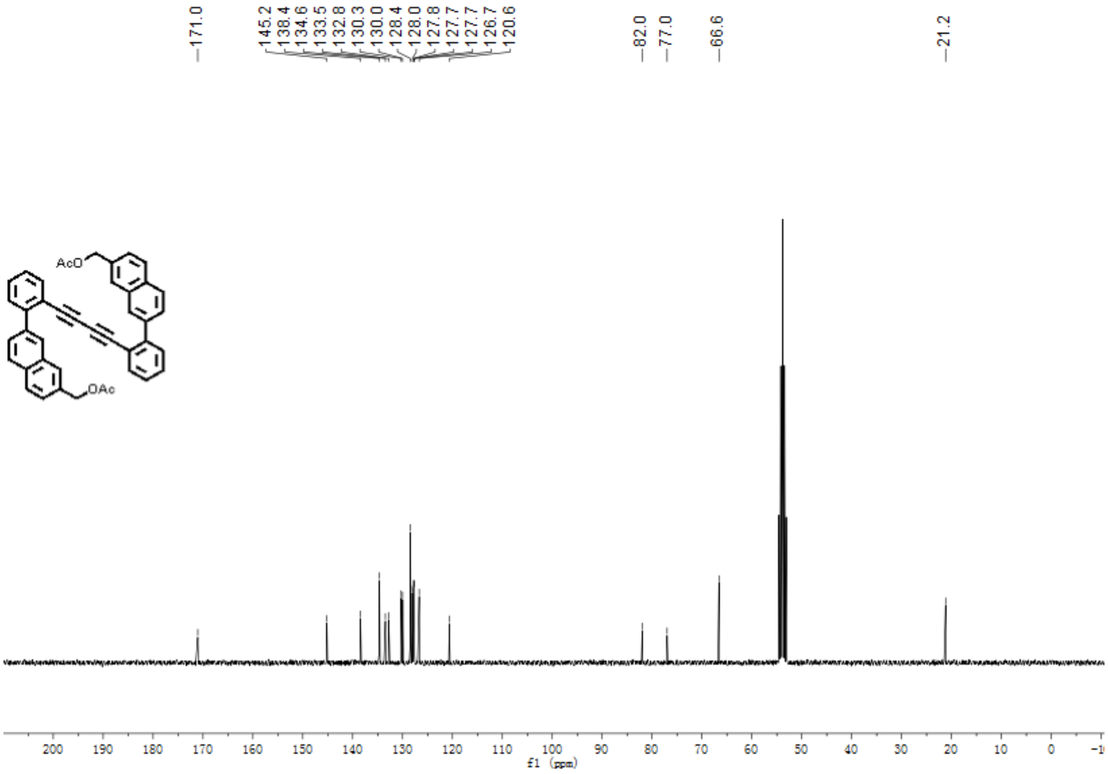


**Figure S8.** $^{13}$ C NMR spectra of compound **6** in $CD_2Cl_2$ (75 MHz, 298 K).

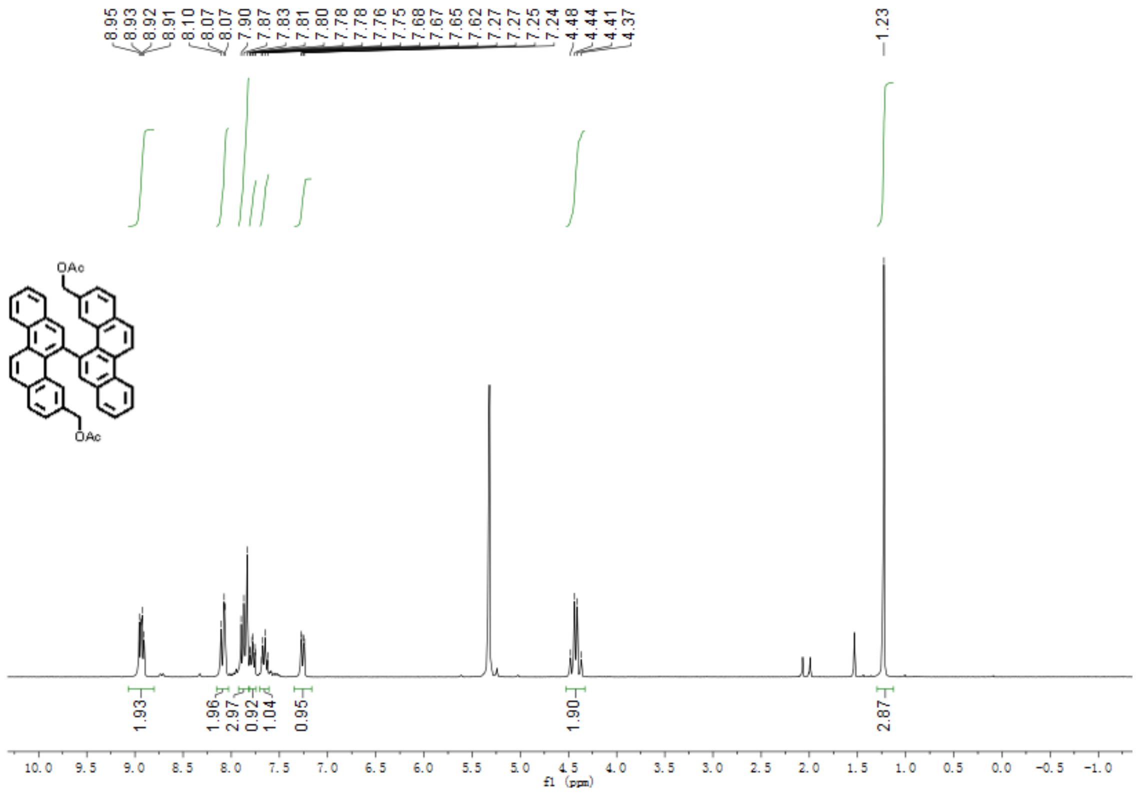

**Figure S9.** $^{1}$H NMR spectra of compound **7** in $CD_2Cl_2$ (300 MHz, 298 K).

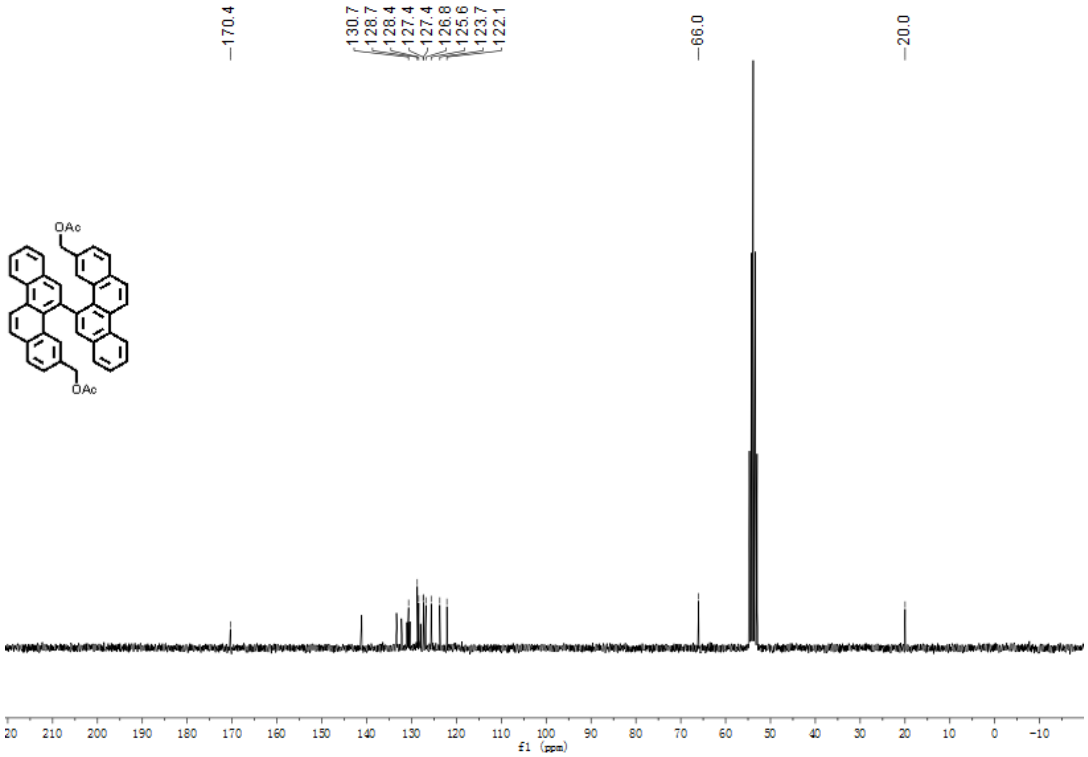

**Figure S10.** $^{13}$ C NMR spectra of compound **7** in $CD_2Cl_2$ (75 MHz, 298 K).

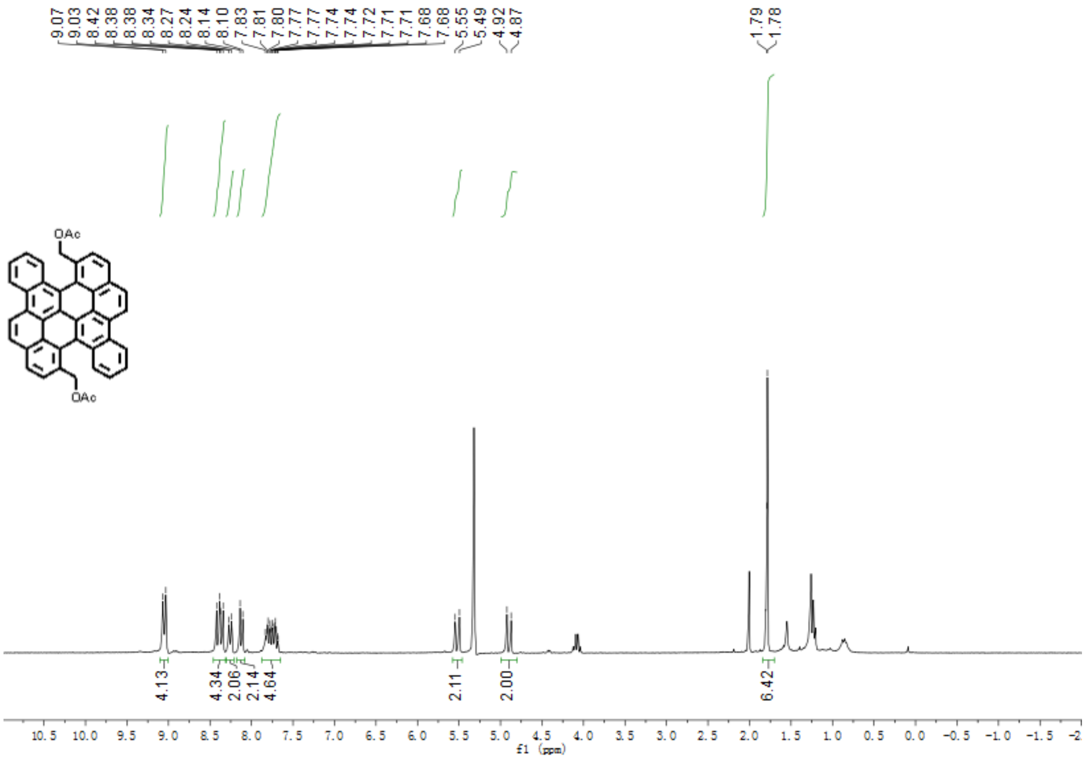


**Figure S11.** $^{1}H$ NMR spectra of compound **8** in $CD_2Cl_2$ (250 MHz, 298 K).

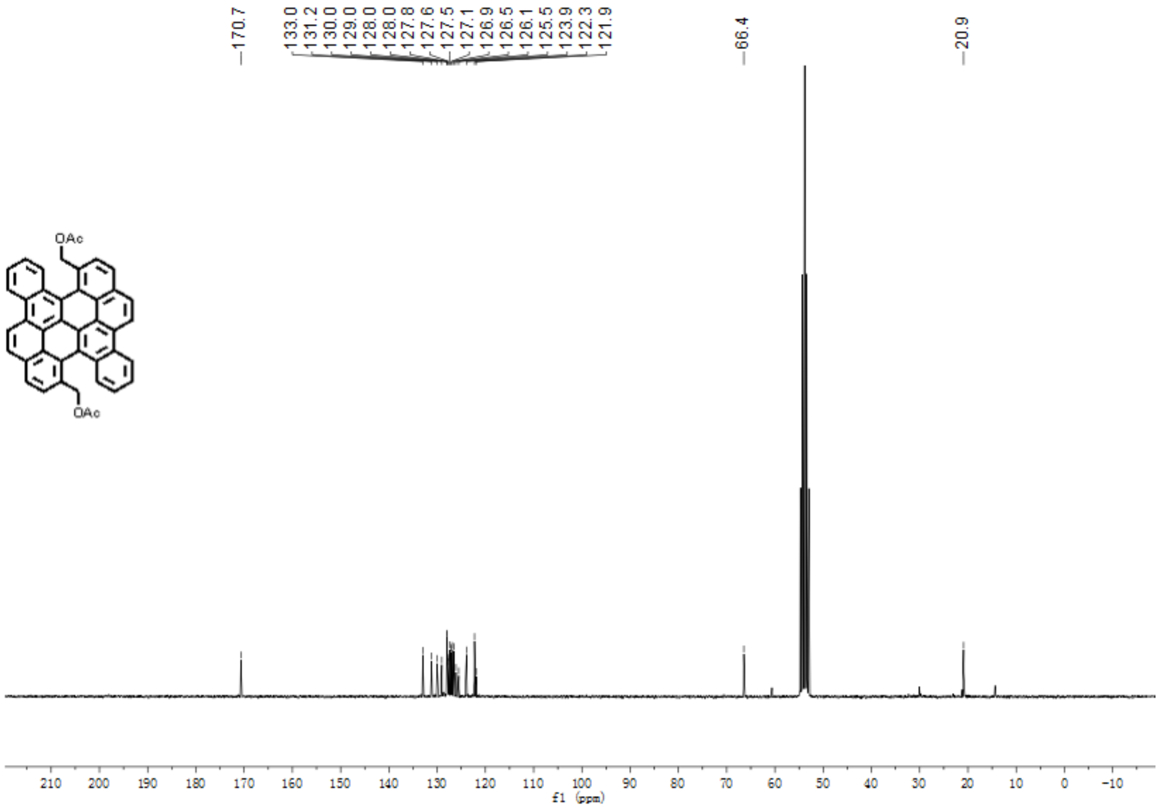


**Figure S12.** $^{13}C$ NMR spectra of compound **8** in $CD_2Cl_2$ (63 MHz, 298 K).

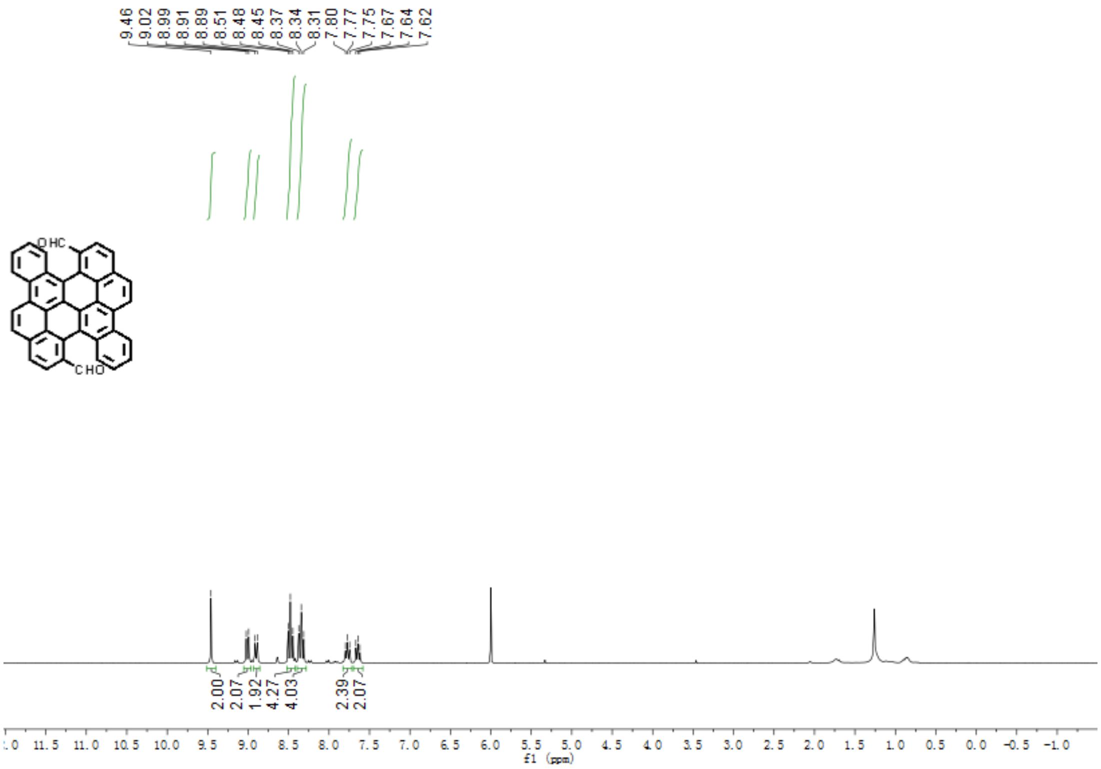


**Figure S13.** $^{1}$H NMR spectra of compound **9** in $C_2D_2Cl_4$ (300 MHz, 298 K).

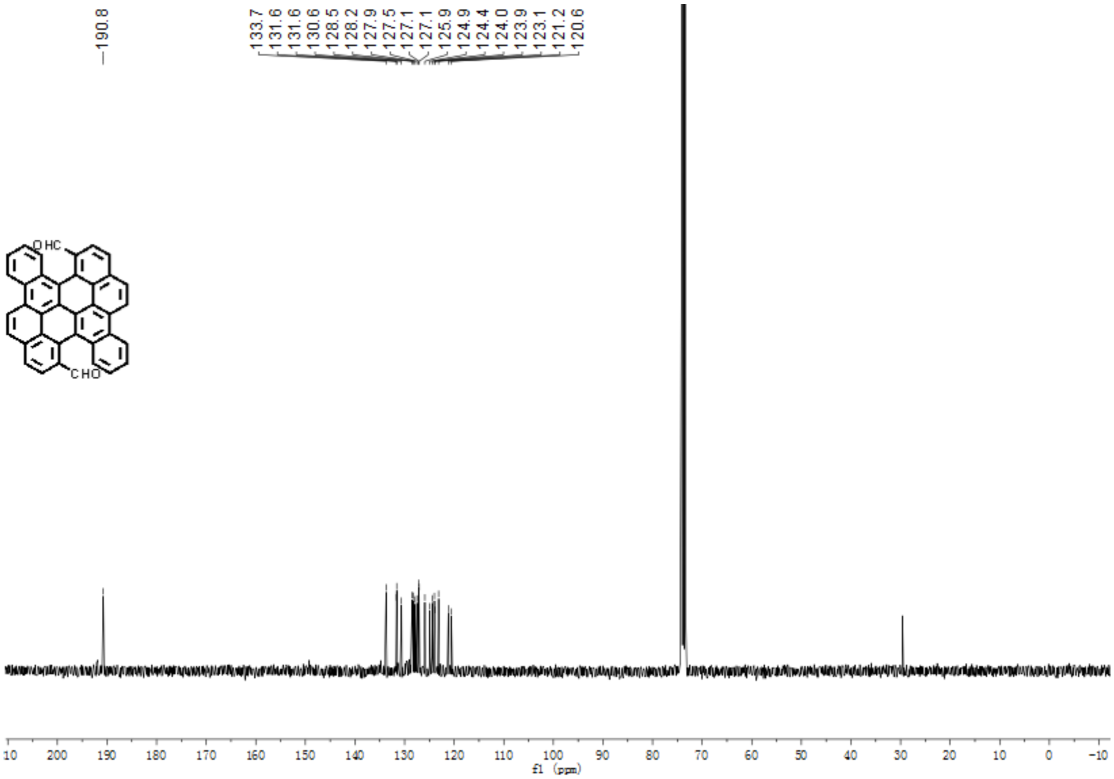


**Figure S14.** $^{13}$C NMR spectra of compound **9** in $C_2D_2Cl_4$ (75 MHz, 298 K).

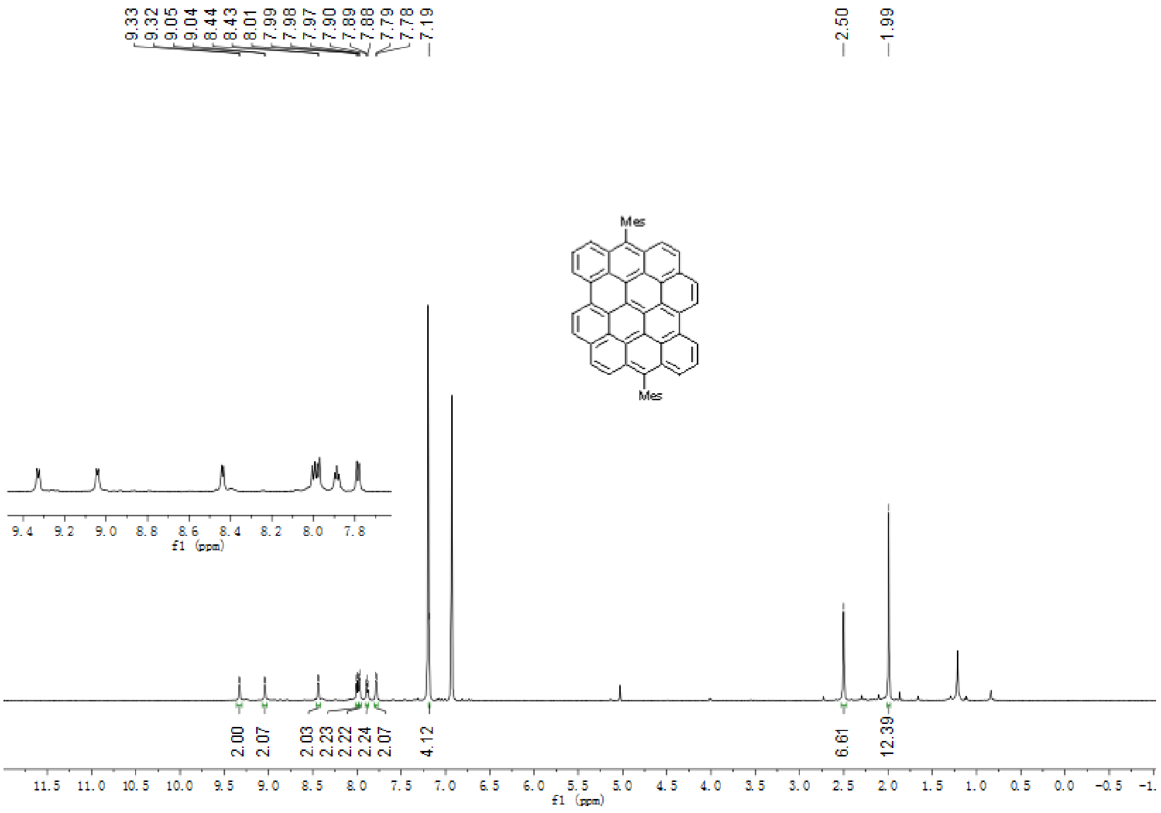


**Figure S15.** $^{1}$H NMR spectra of DBOV-Mes in *o*-dichlorobenzene ($d_6$) (700 MHz, 343 K).

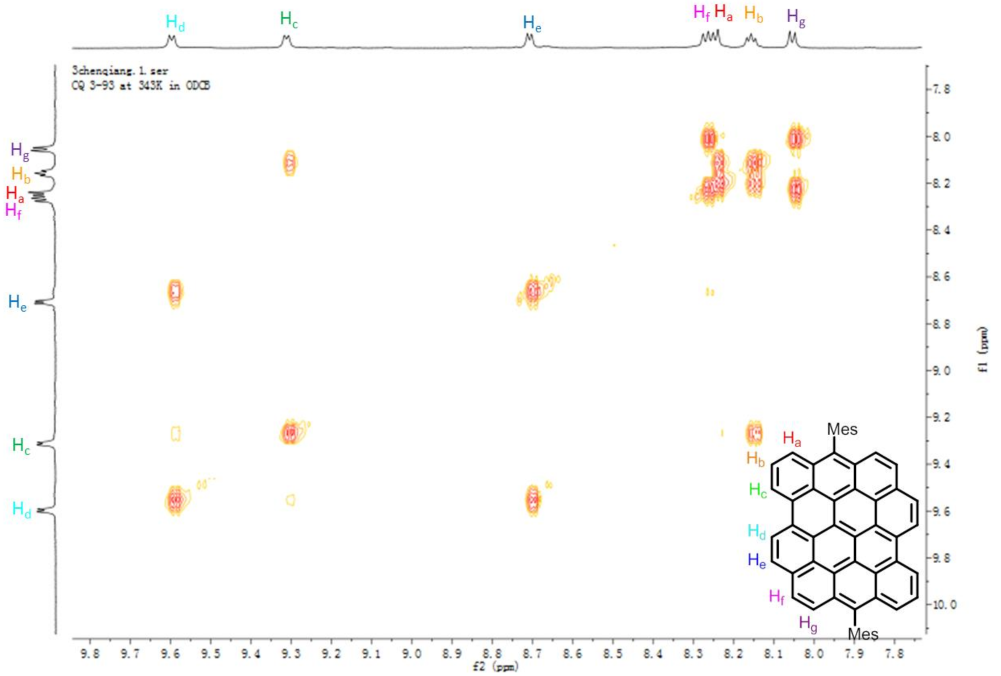


**Figure S16.** H-H COSY spectra of DBOV-Mes in *o*-dichlorobenzene ($d_6$) (700 MHz, 343 K).

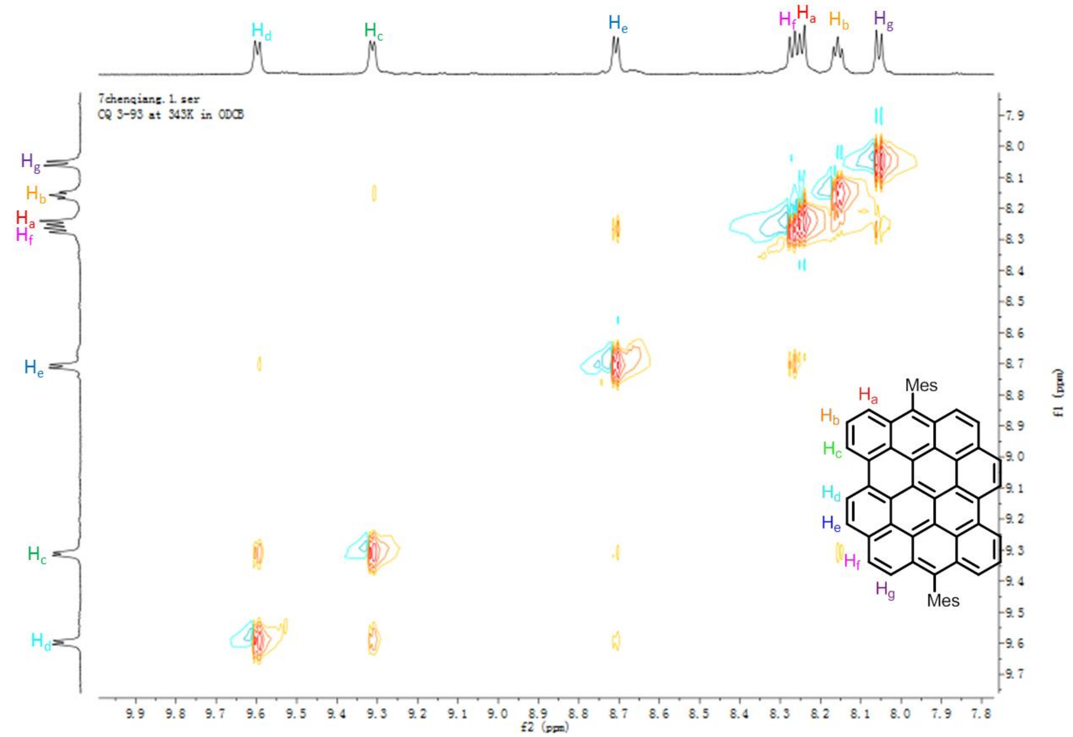


**Figure S17.** NOESY spectra of DBOV-Mes in *o*-dichlorobenzene ($d_6$) (700 MHz, 343 K).

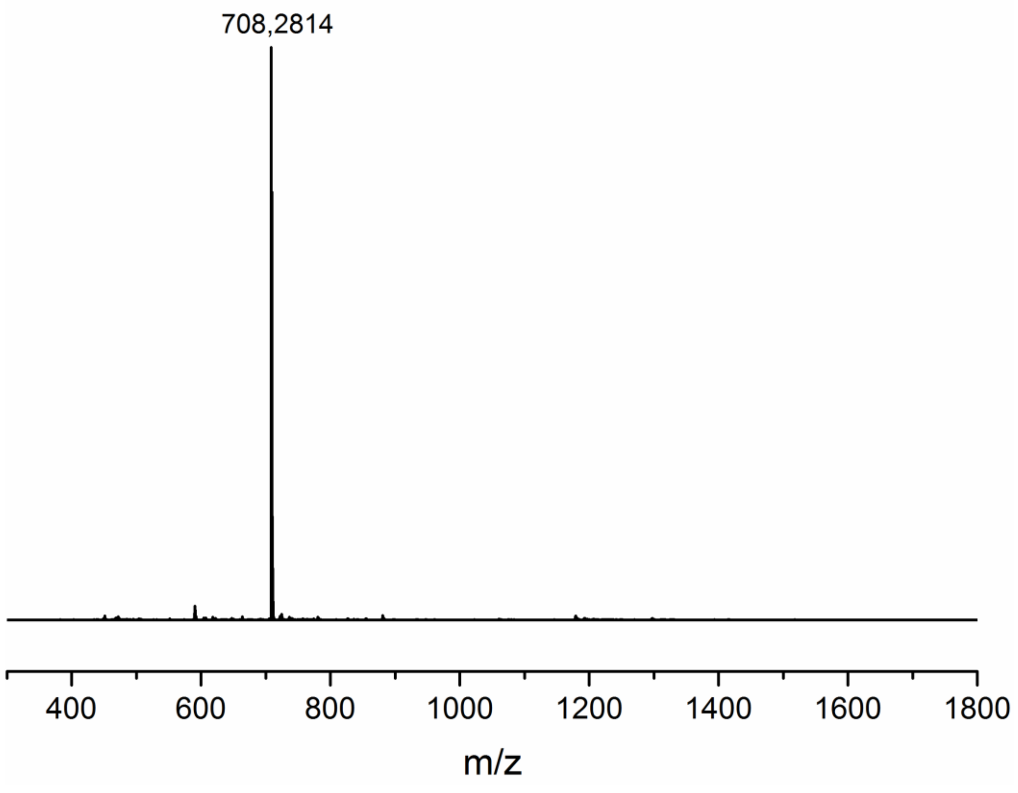


**Figure S18.** HR MALDI-TOF MS spectra of **DBOV-Mes**.

## References

1. T. Dumslaff, B. Yang, A. Maghsoumi, G. Velpula, K. S. Mali, C. Castiglioni, S. D. Feyter, M. Tommasini, A. Narita, X. Feng, and K. Müllen, *J. Am. Chem. Soc.* **2016** 138 (14), 4726-4729.

2. G. M. Paterno, Q. Chen, X.-Y. Wang, J. Liu, S. G. Motti, A. Petrozza, X. Feng, G. Lanzani, K. Müllen, A. Narita, and F. Scotognella, *Angew. Chem. Int. Ed.*, **2017**, DOI: 10.1002/anie.201700730
